# Supplementary material for: Conversational Information Seeking
Source: arXiv:2201.08808 source file (2023-01-25)
Supplement: Supplementary file 2 [file appendix2.tex]

\chapter{Datasets}
\label{appendixB}

\todo{We'll dump citations for datasets and other resources here, and will decide at a later date if we actually want to write it.}

One idea: Go through all the citations \& make a big list of the \emph{public} datasets they use. We'd then cross-reference how the datasets are used by theme (section?), solving the problem of how to select which datasets we cover.

\begin{itemize}
\item \cite{Penha:2019:MANtIS} has a nice table comparing this and other datasets.
\item \cite{Serban:2018:Corpora} is another good source.
\end{itemize}
